# Supplementary material for: On monitoring development indicators using high resolution satellite images
Source: arXiv:1712.02282 source file (2018-06-25)
Supplement: Supplementary file 1 [file appendix.tex]

\appendix
\section{Night light data}
\label{sec:nightlight}
